# Supplementary material for: Concise and interpretable multi-label rule sets
Source: arXiv:2210.01533 source file (2022-11-07)
Supplement: Supplementary file 1 [file appendix_other_metrics.tex]

\section{Experiment Results: Other Metrics}
\begin{table*}\vspace*{-5cm}
	\centering
	\begin{tabular}{||c c c c c c c c||}
		\hline
		Dataset &  DMRS & \seco & Boomer (10)  & Boomer (100) & Boomer (1000) & BR-SVM \\ [0.25ex] 
		\hline\hline
		\textsc{\enron} & 0.21 & NA & 0.025 & 0.040 & 0.116 & 0.22   \\ 
		\hline
		\textsc{\medical} & 0.88 & 0.35 &  0.0 & 0.076 & 0.30 & 0.99   \\ 
		\hline
		\textsc{\CAL}& 0.47 & NA & 0.0790 & 0.210 & 0.583 & 0.49  \\ 
		\hline 
		\textsc{\bibtex} & 0.2 & NA & 0.0 & 0.0 & 0.036 & 0.30   \\ 
		\hline 
		\textsc{\emotions}& 0.6 & 0.529 & 0.55 & 0.57 & 0.557 & 0.6   \\ 
		\hline
		\textsc{\mediamill} & 0.051 & NA & 0.016 & 0.016 & 0.0164 & 0.04   \\ 
		\hline 
		\textsc{\birds} & 0.295 & 0.314 & 0.032 & 0.184 & 0.393 & 0.30  \\ [1ex] 
		\hline
	\end{tabular}
	\caption{\label{tab:macrof1scoresBoomer} Real data. Macro-averaged $F_1$-score for our approach, \Boomer with increasing number of rules, and \SVM. }
\end{table*}
\begin{table*}\vspace*{-15cm}
	\centering
	\begin{tabular}{||c c c c c c c c||}
		\hline
		Dataset &  DMRS & \seco & Boomer (10)  & Boomer (100) & Boomer (1000) & BR-SVM  \\ [0.25ex] 
		\hline\hline
		\textsc{\enron} & 0.94 & NA &  0.9376 & 0.943 & 0.954 & 0.95  \\
		\hline
		\textsc{\medical}  & 0.99 & 0.979 & 0.972 &  0.973 & 0.98 & 0.99  \\
		\hline
		\textsc{\CAL} & 0.87 & NA &  0.836 & 0.855 & 0.904 & 0.87  \\
		\hline 
		\textsc{\bibtex}   & 0.987 & NA &  0.9846 &  0.985 &  0.986 & 0.98   \\
		\hline 
		\textsc{\emotions} & 0.69 & 0.70 & 0.73 & 0.76 & 0.75 & 0.74   \\
		\hline
		\textsc{\mediamill}  & 0.962 & NA & 0.964 & 0.964 &  0.965 & 0.97   \\ 
		\hline 
		\textsc{\birds}  & 0.941 & 0.941 & 0.949 & 0.952 & 0.952 &  0.94   \\ [1ex] 
		\hline
	\end{tabular}
	\caption{\label{tab:f1scoresBoomer} Real data. Hamming score for our approach, \Boomer with increasing number of rules, and \SVM. }
\end{table*}
